# Supplementary material for: Tenplex: Dynamic Parallelism for Deep Learning using Parallelizable Tensor Collections
Source: arXiv:2312.05181 source file (2024-09-26)
Supplement: Supplementary file 1 [file appendix.tex]

% Appendix

\section{PTC formalization}

\subsection{Parallelizations}
\label{sec:ptc:parallelizations}

Next, we show how a PTC represents multi-dimensional parallelization configurations (\ie data, model, and pipeline parallelism) by using different slicing functions~$\sigma$, partitioning functions~$\phi$, and allocation functions~$\alpha$. We assume a $n$-parameter model, $M = (t_1, \dots, t_n)$, a $m$-sample dataset, $D = (t_{n+1}, \dots, t_{n+m})$, and $k$~GPU devices, $R = (r_1, \dots, r_k)$:

\myparr{Data parallelism~(DP)} replicates the model and partitions the data samples across $k$~GPUs. This means that $M$ and $D$ are not sliced, $\sigma(t) = \{t\}, \forall t \in M \cup D$ and $U = \{\{t_1\}, \dots, \{t_{n+m}\}\}$. The partitioning function $\phi$ groups the model together as one sub-collection, and each data partition as a sub-collection, $\phi(U) = \{S_1, \dots, S_{k+1}\}$, where $S_1 = M$ and $S_2$ to $S_{k+1}$ are the data sub-collections.

Finally, the allocation function~$\alpha$ assigns the model sub-collections to all $k$~GPUs, $\alpha(S_1) = \{r_1, \dots, r_k\}$. It assigns the data sub-collections across $k$~GPUs, $\alpha(S_{i+1}) = \{r_{i}\}, \forall S_i \in S, 1\le i \le k$. In practice, a DL job trains models on data batches, therefore, $\phi$ and $\alpha$ are applied to each batch.

\myparr{Model parallelism~(MP)} slices each tensor of model parameters into $k$~sub-tensors, $\sigma(t) = \{t^1, \dots, t^k\}, \forall t \in M$. In contrast, the dataset~$D$ is not sliced, $\sigma(t) = \{t\}, \forall t \in D$. The sub-tensor collection is $U = \{\{t_1^1, \dots, t_1^k\}, \dots, \{t_n^1, \dots, t_n^k\}, \{t_{n+1}\}, \dots \{t_{n+m}\}\}$. 

The partitioning function~$\phi$ then groups the sub-tensors to $k+1$~sub-collections, $\phi(U) = \{S_1, \dots, S_{k+1}\}$, while ensuring a sub-collection has one sub-tensor of each parameter, $S_i=\{t_1^i \dots t_n^i\}, 1\le i \le k$. The dataset tensors form $S_{k+1}$. The allocation function~$\alpha$ assigns each model sub-collection to a GPU, $\alpha(S_i) = \{r_i\}, 1\le i \le k$, while distributing the whole dataset to all GPU devices, $\alpha(S_{k+1}) = \{r_1, \dots, r_k\}$.

\myparr{Pipeline parallelism~(PP)} partitions sets of \emph{layers} and allocates them across $k$~GPUs. It does not slice model tensors nor the dataset, $\sigma(t) = \{t\}, \forall t \in D \cup M$, but partitions these tensors into $k$~sets of layers, $\phi(U)=\{S_1,\dots, S_{k+1}\}$.

The partitioning function is defined in the parallelization configuration. Without loss of generality, we assume that layers are evenly partitioned, and each layer has the same number of parameters: $\phi$ maps $t_i$ to $S_j$ where $j = \lfloor \frac{i}{\lceil n/k \rceil} \rfloor$. $S_{k+1} = D$ for the dataset. Data samples are only needed at the first layer as the input and the last layer to compute the loss value, $\alpha(S_{k+1})=\{r_1, r_k\}$. The model sub-collections are allocated to one GPU, $\alpha(S_i) = \{r_i\}, 1\le i \le k$.

% End
